# Supplementary material for: Engineering Nonlinear Response of Superconducting Niobium Microstrip Resonators via Aluminum Cladding
Source: arXiv:1811.09170 source file (2019-10-15)
Supplement: Supplementary file 1 [file supp.pdf]

# Engineering Nonlinear Response of Superconducting Niobium Microstrip Resonators via Aluminum Cladding: Supplementary Material

Sangil Kwon[1,2], Yong-Chao Tang[1,3], Hamid R. Mohebbi[4], Olaf W. B. Benningshof[1,2], David G. Cory[1,5,6,7], and Guo-Xing Miao[1,3]

[1] *Institute for Quantum Computing, University of Waterloo, Waterloo, Ontario N2L 3G1, Canada*
[2] *Department of Physics and Astronomy, University of Waterloo, Waterloo, Ontario N2L 3G1, Canada*
[3] *Department of Electrical and Computer Engineering, University of Waterloo, Waterloo, Ontario N2L 3G1, Canada*
[4] *High Q Technologies LP, Waterloo, Ontario N2L 0A7, Canada*
[5] *Department of Chemistry, University of Waterloo, Waterloo, Ontario N2L 3G1, Canada*
[6] *Perimeter Institute for Theoretical Physics, Waterloo, Ontario N2L 2Y5, Canada*
[7] *Canada Institute for Advanced Research, Toronto, Ontario M5G 1Z8, Canada*

## S1 Anisotropic Ginzburg–Landau Equations

The anisotropic Ginzburg–Landau (GL) equations are given by (in SI units) [1]

$$\alpha\psi + \beta|\psi|^2\psi + \frac{1}{2}\left(\frac{\hbar}{i}\nabla - e_\mathrm{s}\vec{A}\right)\cdot\left[\frac{1}{m^*}\right]\cdot\left(\frac{\hbar}{i}\nabla - e_\mathrm{s}\vec{A}\right)\psi = 0, \tag{S1}$$

$$\frac{1}{\mu_0}\nabla\times\nabla\times\vec{A} = \frac{e_\mathrm{s}\hbar}{2i}\left[\frac{1}{m^*}\right]\cdot\left(\psi^*\nabla\psi - \psi\nabla\psi^*\right) - e_\mathrm{s}^2|\psi|^2\left[\frac{1}{m^*}\right]\cdot\vec{A}, \tag{S2}$$

where $\psi = \psi(x, y, z, t)$ is the complex order parameter; $\alpha$ and $\beta$ are phenomenological parameters; $e_\mathrm{s}$ is the charge of the superconducting electron; $\vec{A}$ is the magnetic vector potential; $\phi$ is the electric potential; and $[1/m^*]$ is the anisotropic effective mass tensor defined by

$$\left[\frac{1}{m^*}\right] = \begin{bmatrix} 1/m_\parallel^* & 0 & 0 \\ 0 & 1/m_\perp^* & 0 \\ 0 & 0 & 1/m_\parallel^* \end{bmatrix}.$$

In the anisotropic GL equations, this anisotropic effective mass is responsible for anisotropy in superconducting parameters. Here, we define the anisotropy parameter $\gamma$ as

$$\gamma = \sqrt{\frac{m_\perp^*}{m_\parallel^*}}.$$

Then, we have the following relations:

$$\frac{\xi_\parallel}{\xi_\perp} = \frac{\lambda_\perp}{\lambda_\parallel} = \frac{H_\mathrm{c2}^\parallel}{H_\mathrm{c2}^\perp} = \gamma.$$

We transform the GL equations into dimensionless quantities by measuring length in units of the in-plane penetration depth $\lambda_\parallel\,(\equiv\sqrt{m_\parallel^*\beta/\mu_0 e_\mathrm{s}^2|\alpha|})$; fields in units of $\sqrt{2}H_\mathrm{c}$, where $H_\mathrm{c}\,(\equiv\sqrt{\alpha^2/\mu_0\beta})$ is the thermodynamic critical field; and order parameter in units of $\psi_0\,(\equiv\sqrt{|\alpha|/\beta})$. After the transformation, we introduced a time-dependent term from the time-dependent GL equations (Eqs. (S7) and (S8) of Ref. [2]) to imitate cooling procedures.

For simplicity, the time-dependent term is assumed isotropic. This can be justified by the argument that we are only interested in the steady-state solutions. Then Eqs. (S1) and (S2) are written as

$$\frac{\partial \psi}{\partial t} = -\left(\frac{i}{\kappa_\parallel}\nabla + \vec{A}\right) \cdot \left[\frac{1}{\Gamma^2}\right] \cdot \left(\frac{i}{\kappa_\parallel}\nabla + \vec{A}\right)\psi + \psi - |\psi|^2\psi, \tag{S3}$$

$$\sigma_{\rm n}\frac{\partial \vec{A}}{\partial t} = \frac{1}{2i\kappa_\parallel}\left[\frac{1}{\Gamma^2}\right] \cdot \left(\psi^*\nabla\psi - \psi\nabla\psi^*\right) - |\psi|^2\left[\frac{1}{\Gamma^2}\right] \cdot \vec{A} - \nabla \times \nabla \times \vec{A}, \tag{S4}$$

where $\kappa_\parallel \equiv \lambda_\parallel/\xi_\parallel$ is the GL parameter; $\sigma_{\rm n}$ is the inverse of the residual resistivity; and $[1/\Gamma^2]$ is a tensor given by

$$\left[\frac{1}{\Gamma^2}\right] = \begin{bmatrix} 1 & 0 & 0 \\ 0 & 1/\gamma^2 & 0 \\ 0 & 0 & 1 \end{bmatrix}.$$

To solve Eqs. (S3) and (S4), we used COMSOL Multiphysics 5.1. The general form of partial differential equations in COMSOL Multiphysics is

$$\mathbf{e}_a\frac{\partial^2 \mathbf{u}}{\partial t^2} + \mathbf{d}_a\frac{\partial \mathbf{u}}{\partial t} + \nabla \cdot \mathbf{\Gamma} = \mathbf{f}. \tag{S5}$$

All geometries were assumed to be two-dimensional systems on the $xy$ plane. The applied magnetic field $\vec{H}_{\rm a}$ is assumed along the $z$ direction. In this case, $\mathbf{u} = (u_1, u_2, u_3, u_4, u_5)^\top$, where $\top$ is the transpose. The variables are given by $u_1(x,y,t) = {\rm Re}(\psi(x,y,t))$, $u_2(x,y,t) = {\rm Im}(\psi(x,y,t))$, $u_3(x,y,t) = A_x(x,y,t)$, and $u_4(x,y,t) = A_y(x,y,t)$, respectively. An auxiliary variable $u_5$ is always zero. In Eq. (S5), $\mathbf{e}_a$ is a zero matrix. Others can be written as

$$\mathbf{d}_a = \begin{bmatrix} 1 & 0 & 0 & 0 & 0 \\ 0 & 1 & 0 & 0 & 0 \\ 0 & 0 & \sigma_{\rm n} & 0 & 0 \\ 0 & 0 & 0 & \sigma_{\rm n} & 0 \\ 0 & 0 & 0 & 0 & 0 \end{bmatrix}, \quad \mathbf{\Gamma} = \begin{bmatrix} [-\partial_x u_1/\kappa_\parallel^2, -\partial_y u_1/(\gamma\kappa_\parallel)^2]^\top \\ [-\partial_x u_2/\kappa_\parallel^2, -\partial_y u_2/(\gamma\kappa_\parallel)^2]^\top \\ [0, \partial_x u_4 - \partial_y u_3 - \mu_0 H_{\rm a}]^\top \\ [-\partial_x u_4 + \partial_y u_3 + \mu_0 H_{\rm a}, 0]^\top \\ [u_3, u_4]^\top \end{bmatrix},$$

$$\mathbf{f} = \begin{bmatrix} (\partial_x u_3 + \partial_y u_4/\gamma^2)u_2/\kappa_\parallel + 2(u_3\partial_x u_2 + u_4\partial_y u_2/\gamma^2)/\kappa_\parallel - (u_3^2 + u_4^2)u_1 + u_1 - (u_1^2 + u_2^2)u_1 \\ -(\partial_x u_3 + \partial_y u_4/\gamma^2)u_1/\kappa_\parallel - 2(u_3\partial_x u_1 + u_4\partial_y u_1/\gamma^2)/\kappa_\parallel - (u_3^2 + u_4^2)u_2 + u_2 - (u_1^2 + u_2^2)u_2 \\ (u_1\partial_x u_2 - u_2\partial_x u_1)/\kappa_\parallel - (u_1^2 + u_2^2)u_3 \\ (u_1\partial_y u_2 - u_2\partial_y u_1)/(\gamma^2\kappa_\parallel) - (u_1^2 + u_2^2)u_4/\gamma^2 \\ \partial_x u_3 + \partial_y u_4 + u_5 \end{bmatrix}.$$

The boundary conditions were implemented using "zero flux" $-\vec{n} \cdot \mathbf{\Gamma} = \mathbf{G}$, where $\mathbf{G} = [0,0,0,0,0]^\top$. The details of this implementation is described in Refs. [2, 3].

# S2 Extracting Loss Parameters from the Parallel Field Data

To extract loss parameters from the parallel field data (Fig. 4 in the main text), we should calculate the expected resonance frequency $f$ and the quality factor $Q$ as a function of external magnetic field $H$. In the following, we introduce some formulas required for those calculations (see Sec. II of Ref. [2] for more information).

The magnetic field dependent parts of $f$ and $Q$ are given by

$$\frac{f^{-2}(H) - f_0^{-2}}{f_0^{-2}} = \frac{L(H) - L_0}{L_0}, \quad \frac{1}{Q(H)} = \frac{P_{\rm diss}(H)}{2\pi f(H) U_{\rm em}(H)}, \tag{S6}$$

where $f_0$ is the resonance frequency at zero-field; $L_{(0)}$ is the effective inductance per unit length (at zero-field); $Q_0$ is the quality factor at zero-field; $P_{\rm diss}$ is the dissipated power per unit length; and $U_{\rm em}$ is the stored electromagnetic energy per unit length. Since $L$ is defined by the relation $U_{\rm em} = L|I|^2/2$, where $I$ is the total microwave current, the quantities we need to calculate are $U_{\rm em}$ and $P_{\rm diss}$.

Consider a microstrip line oriented along the $z$ axis with its width along the $x$ axis and thickness along the $y$ axis. In this configuration, $U_{\rm em}$ is defined by

$$U_{\rm em}(H) = \frac{1}{2}\int_{\rm all} \mu_0 |H_{\rm mw}(x,y,\lambda(H))|^2 dxdy + \frac{1}{2}\int_{\rm sc} \frac{\rho_2(x,y,H)}{\omega} |J_{\rm mw}(x,y,\lambda(H))|^2 dxdy \tag{S7}$$

where $\mu_0$ is the vacuum permeability; $\rho$ is the complex resistivity $\rho_1 + {\rm i}\rho_2$; $H_{\rm mw}$ is the microwave magnetic field strength; $J_{\rm mw}$ is the microwave current density; $\lambda$ is the penetration depth; $\omega/2\pi$ is the frequency of an applied electromagnetic field; and "sc" stands for "inside superconducting media". Next, $P_{\rm diss}$ is defined by

$$P_{\rm diss}(H) = \frac{1}{2}\int_{\rm sc} \rho_1(x,y,H) |J_{\rm mw}(x,y,\lambda(H))|^2 dxdy. \tag{S8}$$

In Eqs. (S7) and (S8), $J_{\rm mw}$ and $H_{\rm mw}$ can be simulated by the Maxwell equations and the London equations (see Sec. S2 of Ref. [2] for details of the simulation). For the complex resistivity, we employ the two-fluid model. The complex conductivity based on the two-fluid model $\sigma_{\rm tf,1} - {\rm i}\sigma_{\rm tf,2}$ is given by [4]

$$\sigma_{\rm tf,1} = \frac{n_{\rm n}}{n_{\rm tot}}\sigma_{\rm n}, \quad \sigma_{\rm tf,2} = \frac{n_{\rm s} {e_{\rm s}}^2}{m_{\rm s}\omega} = \frac{1}{\omega\mu_0\lambda^2}, \tag{S9}$$

where $n_{\rm s}$ is the local number density of superconducting electrons; $n_{\rm n}$ is the local number density of normal electrons; $n_{\rm tot}$ is the total number density of conduction electrons; $\sigma_{\rm n}$ is the inverse of the residual resistivity $\rho_{\rm n}$; $e_{\rm s}$ is the charge of a superconducting electron; and $m_{\rm s}$ is the mass of a superconducting electron. The corresponding complex resistivity $\rho_{\rm tf}$ is given by $\rho_{{\rm tf},i} = \sigma_{{\rm tf},i}/(\sigma_{\rm tf,1}^2 + \sigma_{\rm tf,2}^2)$.

Once we solve the anisotropic GL equations as described in Sec. S1, $n_{\rm s}$ can be calculated using the relation $n_{\rm s}(x,y,H) = |\psi(x,y,H)|^2$. As the GL theory does not give $n_{\rm n}$, we introduce an empirical expression for $n_{\rm n}$ with an additional exponent $\beta$:

$$\frac{n_{\rm n}(H)}{n_{\rm tot}} = \left[1 - \frac{n_{\rm s}(H)}{n_{\rm s}(0)}\right]^{\beta}. \tag{S10}$$

The procedure for extracting the loss parameters used in this work is identical to that in Ref. [2], except two parameters, $\lambda_0$ and $\kappa$ in Ref. [2], become $\lambda_0^{\parallel}$ and $\gamma\kappa_{\parallel}$ due to the anisotropy. A brief description of the procedure is as follows (see Sec. S3 of Ref. [2] for more details):

1. Calculate $n_{\rm s}$ as a function of $H_{\parallel}$ by solving the GL equations; $\lambda_0^{\parallel}$ and $\gamma\kappa_{\parallel}$ are required for this step.
2. Since $n_{\rm s} \propto \lambda^{-2}$ [Eq. (S9)], $\lambda_{\parallel}(H_{\parallel})$ is obtained by $(\lambda_0^{\parallel}/\lambda_{\parallel})^2 = n_{\rm s}(H_{\parallel})/n_{\rm s}(0)$. Once $\lambda_{\parallel}$ is known, $J_{\rm mw}$ and $H_{\rm mw}$ can be simulated. Here, note that $\lambda_{\parallel}$ is responsible for those simulations because the microwave current flows parallel to the film.
3. $f^{-2}$ is reconstructed theoretically using Eqs. (S6), (S7), and (S9); $H_{\rm c}$ is required for this step.
4. Repeat steps 1–3 until the theoretical $f^{-2}$ is sufficiently close to the experimental results. Then, $\lambda_0^{\parallel}$, $\gamma\kappa_{\parallel}$, and $H_{\rm c}$ are determined. Here, $\lambda_0^{\parallel}$ is determined by the slope of $f^{-2}(H_{\parallel})$ below $H_{\rm vp}^{\parallel}$ because the slope of $f^{-2}(H_{\parallel})$ was determined primarily by geometrical constriction, given by $d/\lambda_0^{\parallel}$, where $d$ is the thickness of the whole trilayer; $\gamma\kappa_{\parallel}$ is chiefly determined by $H_{\rm vp}^{\parallel}$.
5. Using $n_{\rm s}(H_{\parallel})$ from the $f^{-2}$ data, $Q_0$, $\beta$, and $\rho_{\rm n}$ are determined by the $Q^{-1}$ data using a similar procedure and Eqs. (S6)–(S10).

During the calculation, as in Ref. [2], the ground plane's contribution to the resonator properties was assumed to be negligible because this contribution to the microwave current density is just a few percent. The same assumption was also applied for the loss parameters associated with vortex motion.

# S3 Magnetic Hysteresis in a Finite Perpendicular Field

As mentioned in Sec. IV, we found that applying a high microwave current in a magnetic field perpendicular to the film $H_\perp$ results in magnetic hysteresis. To explore the effect of $H_\perp$ on the nonlinear behavior, which will be crucial for resonators misaligned with the field, we measured the microwave power dependence of Al-5L with a finite $H_\perp$.

$H_\perp$ was applied by tilting the resonator in a background magnetic field parallel to the microwave current $H_{\rm bg}$ using the goniometer mentioned in Sec. II. $H_\perp$ is obtained by $H_\perp = H_{\rm bg}\sin\theta$, where $\theta$ is the tilt angle. In this work, $\mu_0 H_{\rm bg} = 0.35$ T. Two different types of cooling procedure were used: zero-field cooling (ZFC) and heat pulsing (HP). For the ZFC procedure, the resonator is cooled without any magnetic field. For the HP procedure, a heat pulse is applied to completely suppress superconductivity, then the resonator is cooled back in field to the target temperature. The HP procedure is used to ensure a uniform vortex distribution and suppress the Meissner current as much as possible such that vortex motion becomes the dominant loss mechanism [2].

After applying a high microwave current, significant changes in $f$ and $Q$ were observed as shown in Fig. S1. These changes at various $H_\perp$ are presented in Fig. S2(a). The data were taken by the following procedure: First, $H_\perp$ is applied after ZFC by tilting the resonator. Then the incident power on the input capacitor of the resonator $P_{\rm in}$ is applied from low power ($-57$ dBm) to the power called the current annealing power $P_{\rm CA}$. Note that as $P_{\rm in}$ increases, the spectrum not only shows the Duffing-like nonlinearity but also shifts to a higher frequency as shown in Fig. S1 (solid lines). Once $P_{\rm in}$ reaches $P_{\rm CA}$ ($-7$ dBm for Fig. S1), $P_{\rm in}$ is reduced to $-57$ dBm. We call the procedure up to this point the initial current annealing. After the initial current annealing, no spectrum shift is observed for $P_{\rm in} \leq P_{\rm CA}$ (dashed lines). The position of the spectrum from a low-power measurement is completely determined by the highest power prior to the low-power measurement regardless of a history of $P_{\rm in}$.

To understand the origin of this hysteresis induced by high microwave current, we first consider the $H_\perp$ dependence of $f^{-2}$ and $Q$ without the current annealing [Fig. S2(a)]. After the HP procedure, $f^{-2}$ and $Q^{-1}$ vary linearly with the field, i.e., $Q$ is roughly proportional to the inverse of $H_\perp$, indicating continuous occupation of vortices [2]. Hence, the magnetic field dependence after the HP procedure is governed by vortex motion. A key feature of the data after the ZFC procedure without current annealing is that an anomaly (peak/dip) appears at the field B (6.7 mT) in the $f^{-2}$ data. As shown in our previous work [2], this frequency anomaly is an indication of complete suppression of the Bean–Livingston type edge barrier [5]; hence, the field B is the vortex penetration field perpendicular to the film $H_{\rm p}^{\perp}$. Below this field, the magnetic field dependences of the microwave properties are governed by quasiparticles generated by the Meissner current; above this field, vortex motion is the dominant mechanism. If a superconducting resonator is in a metastable state due to the edge barrier, the high microwave current can change the resonator state via suppressing the edge barrier [6], resulting in different $f$ and $Q$ values. This suppression of the edge barrier by the microwave current is indeed indicated by the result in Fig. S2(a) that the frequency anomaly becomes weaker as $P_{\rm CA}$ increases.

To reveal the physical processes behind the magnetic hysteresis, we use a plot of $Q$ vs. $f^{-2}$ [Fig. S2(b)]. The motivation of this plot is to represent the characteristic relation between the real and imaginary parts of the complex resistivity for each contribution—either quasiparticle generation or vortex motion [2]. In this plot, a process of varying quasiparticle numbers evolves horizontally keeping $Q^{-1}$ constant (an arrow labeled "qp"), while a process of varying vortex numbers evolves as a nearly vertical line (an arrow labeled "vm"). The reason is that, for our device in the range of magnetic fields studied, quasiparticle generation is a very inductive process such that $Q$ is dominated by vortex motion.

Based on this, arrows labeled A, B, and C in Fig. S2(b) suggest that the following processes occur during current annealing [Fig. S2(c)]: (i) At the field A, the edge barrier is suppressed by the microwave current; consequently, vortices penetrate into the resonator. The number of newly injected vortices is not, however, enough to yield a notable change in the Meissner current. (ii) At the field B, a large number of vortices penetrate; as a result, the Meissner current is expelled, i.e., the number of quasiparticles is reduced, by the interaction with the newly injected vortices. These processes result in a reduction of $Q$ and $f^{-2}$, respectively. (iii) At and above the field C, the number of vortices stays similar because the edge barrier is already completely suppressed by $H_\perp$; the Meissner current is expelled notably. This is due to the enhancement of the kinetic energy of existing vortices by the microwave current, or a "shaking" of the vortices. The displacement of vortices during the shaking expels the Meissner current.

In conclusion, we analyzed magnetic hysteresis in $f$ and $Q$ induced by a high microwave current when $H_\perp$ was higher than a certain level. We revealed the physical processes behind this using a plot of $Q$ vs. $f^{-2}$. By doing this, we found that the observed hysteresis was induced by suppression of the edge barrier and consequent vortex injection.

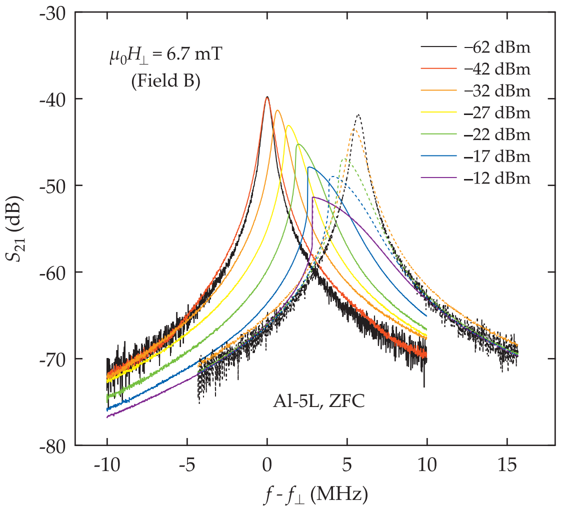


Figure S1: $S_{21}$ curve shift of Al-5L due to a strong microwave current at $\mu_0 H_\perp = 6.7$ mT. Annotated powers ($P_{\mathrm{in}}$) were applied sequentially. $f_\perp$ is the resonance frequency before the initial current annealing. Solid lines are the results from the initial current annealing and dashed lines are from the second annealing. Results from further sequences are identical to the second one. The sweep direction was from low to high frequency. The meaning of the annotation "Field B" can be found in Fig. S2(a). The measurement temperature was about 0.2 K.

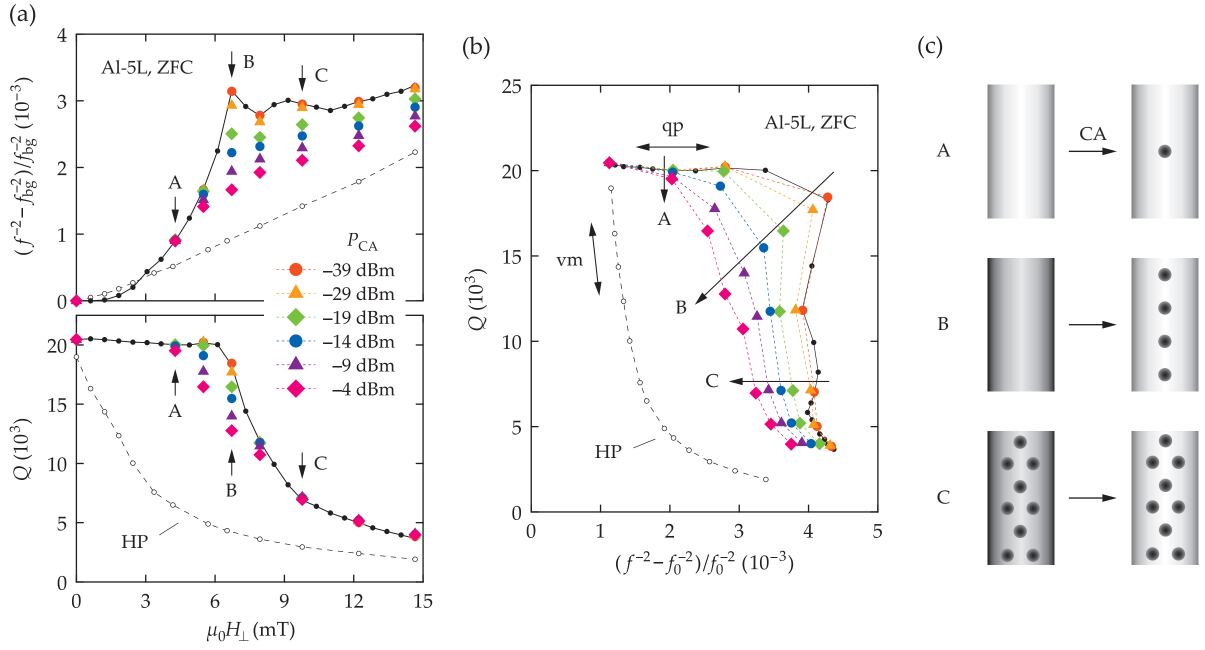


Figure S2: (a) Final $f^{-2}$ and $Q$ for Al-5L measured with $P_{\mathrm{in}} = -57$ dBm after the initial current annealing. (b) A $Q$ vs. $f^{-2}$ plot of the data in (a). Arrows labeled A, B, and C indicate the direction of evolution by the current annealing. In (a,b), symbols with different colors mean that the data were taken with a different $P_{\mathrm{CA}}$, while small black circles were taken without current annealing; small empty circles were taken after the HP procedure. All lines are guides to the eye. (c) The Meissner current and vortices configuration before and after the current annealing at the designated fields. The gray gradient indicates the schematic distribution of the Meissner current density; the darker area is higher current density. The dark gray circles are vortices. The measurement temperature was about 0.2 K.

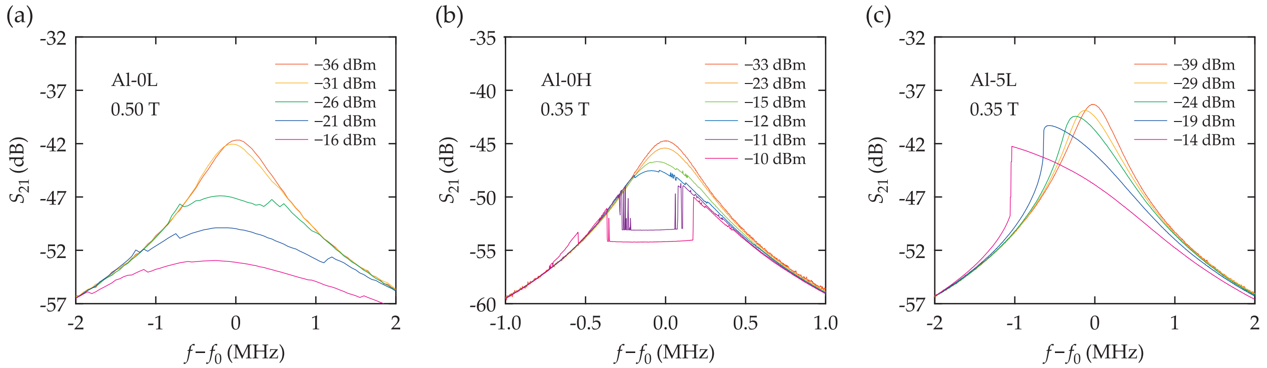


Figure S3: $S_{21}$ resonance curves at various $P_{\text{in}}$ in a modest $H_{\|}$. The sweep direction was from low to high frequency. The measurement temperature was about 0.2 K.

# References


[1] T. Matsushita, *Flux Pinning in Superconductors*, 2nd ed. (Springer, 2014).

[2] S. Kwon, A. Fadavi Roudsari, O. W. B. Benningshof, Y.-C Tang, H. R. Mohebbi, I. A. J. Taminiau, D. Langenberg, S. Lee, G. Nichols, D. G. Cory, and G.-X. Miao, *Magnetic Field Dependent Microwave Losses in Superconducting Niobium Microstrip Resonators*, J. Appl. Phys. **124**, 033903 (2018).

[3] T. S. Alstrøm, M. P. Sørensen, N. F. Pedersen, and S. Madsen, *Magnetic Flux Lines in Complex Geometry Type-II Superconductors Studied by the Time Dependent Ginzburg–Landau Equation*, Acta. Appl. Math. **115**, 63 (2011).

[4] M. Tinkham, *Introduction to Superconductivity*, 2nd ed. (McGraw-Hill, 1996).

[5] C. P. Bean and J. D. Livingston, *Surface Barrier in Type-II Superconductors*, Phys. Rev. Lett. **12**, 14 (1964).

[6] F. Tafuri, J. R. Kirtley, D. Born, D. Stornaiuolo, P. G. Medaglia, P. Orgiani, G. Balestrino, and V. G. Kogan, *Dissipation in Ultra-Thin Current-Carrying Superconducting Bridges; Evidence for Quantum Tunneling of Pearl Vortices*, Europhys. Lett. **73**, 948 (2006).

[7] Y.-C. Tang, S. Kwon, H. R. Mohebbi, D. G. Cory, and G.-X. Miao, *Phonon Engineering in Proximity Enhanced Superconductor Heterostructures*, Sci. Rep. **7**, 4282 (2017).
